# Supplementary material for: Multi-scale and Cross-scale Contrastive Learning for Semantic Segmentation
Source: arXiv:2203.13409 source file (2022-07-19)
Supplement: Supplementary file 1 [file pascal_supp.tex]

% \begin{table*}[htb]
%   \centering
  
% \resizebox{0.6\linewidth}{!}{
%   \begin{tabular}{*6c}
%     \toprule
%     \multicolumn{3}{c}{Network}    & \mc{Loss}                   & \multicolumn{2}{c}{mIoU (ms)}  \\ 
    
%     \cmidrule(r){1-3}               \cmidrule(){4-4}              \cmidrule(l){5-6}  
    
%     \tbf{Model}      & \tbf{Backbone}  &\tbf{Source}          & \quad            & \quad           & Improvement \\
    
%     \midrule    

%     % \hrn             & \mc{HR$48$v$2$} & \cite{mmseg}       & \mc{CE}          & \mc{53.5}       & \quad    \\ 
%     \hrn             & \mc{HR$48$v$2$} & -                  & \mc{CE}          & \mc{53.5}       & \quad    \\ 
%     \hrn             & \mc{HR$48$v$2$} & \cite{HRNet}       & \mc{CE}          & \mc{54.0}       & \quad    \\ 
%     \hrn             & \mc{HR$48$v$2$} & -                  & \mc{ours}        & \mc{\textbf{55.3}}       & $\color{green}(+1.3)$ \\
%     \midrule
%     \hrn             & \mc{HR$48$v$2$} & \cite{exploring_contrastive} & \mc{$\Lc_{c}$+Mem}        & \mc{55.1}       & \quad    \\
%     \midrule    
%     \mc{OCRNet}      & \mc{HR$48$v$2$} & -                  & \mc{CE}          & \mc{56.1}       & \quad    \\ 
%     \mc{OCRNet}      & \mc{HR$48$v$2$} & -                  & \mc{CE}          & \mc{55.8}       & \quad    \\ 
%     \mc{OCRNet}      & \mc{HR$48$v$2$} & \cite{OCR}         & \mc{CE}          & \mc{56.2}       & \quad    \\ 
%     \mc{OCRNet}      & \mc{HR$48$v$2$} & -                  & \mc{ours}        & \mc{56.5}       & $\color{green}(+0.3)$ \\ 
%     \midrule
%     \mc{OCRNet}      & \mc{HR$48$v$2$} & \cite{exploring_contrastive} & \mc{$\Lc_{c}$+Mem}       & \mc{\textbf{57.2}}       & \quad    \\

%     \bottomrule
%   \end{tabular}
  
%   } % resizebox  
%   \caption{Comparisons on \textbf{Pascal-context val} with multi-scale evaluation (ms).}
%   \label{tab:sota_pascal_supp} 
% \end{table*}
